# Supplementary material for: Online Partial Service Hosting at the Edge
Source: arXiv:2103.00555 source file (2022-07-19)
Supplement: Supplementary file 1 [file appendix.tex]

\appendix
\section{Efficient RetroRenting}
We now discuss Efficient RetroRenting (E-RR) (Algorithm \ref{algo:RRE}), an efficient implementation of RR. 
Let $\underbar{\text{$x$}}_t$ = $\min \{x_t, \kappa\}$.
We maintain a quantity $\Delta(t)$, defined as follows:
\begin{align}\label{eq:recursive}
\Delta(t)=\min\Big\{M,\max\big\{0,\Delta(t-1)+\underbar{\text{$x$}}_t-c_t\big\}\Big\},
\end{align}
for $t\geq 1$ and $\Delta(0)=0$. Note that $\Delta(t)\in [0, M].$
In our next result, we show that Algorithms \ref{algo:RR} and \ref{algo:RRE} are equivalent.
\begin{lemma}\label{lem:RR_RRE}
	Algorithms \ref{algo:RR} and \ref{algo:RRE} are equivalent.
\end{lemma}
\begin{proof}
	Let $r_t^{\text{RR}}$  and $r_t^{\text{E-RR}}$ denote the renting variables in time-slot $t$ associated with Algorithms \ref{algo:RR} and \ref{algo:RRE} respectively.
	We have $r_1^{\text{RR}}=r_1^{\text{E-RR}}=0$. Let E-RR fetch the service after the end of time-slot $m$ for the first time. Therefore by Algorithm \ref{algo:RRE},
	$\Delta(t)<M$ for $1\leq t\leq m-1$ and $\Delta(m)=M$, i.e.,
	\begin{align}\label{ineq:fetch_RRE1}
	\Delta(m-1)+\underbar{\text{$x$}}_m-c_m\geq M.
	\end{align}
	Since $\Delta(t)<M$ for $1\leq t\leq m-1$, by \eqref{eq:recursive},    $\Delta(t)=\max\big\{0,  \Delta(t-1)+\underbar{\text{$x$}}_t-c_t\big\}$ for $1\leq t\leq m-1$.
	Let $i \in [1, m-1]$ be a time-slot such that $\Delta(i)=0$ and $\Delta(t)\neq 0$ for $i+1 \leq t<m$. Then, $\Delta(m-1)=\displaystyle\sum_{l=i+1}^{m-1} (\underbar{\text{$x$}}_l-c_l).$
	%Since $\Delta(t)<M$ for $1\leq t\leq m-1$, by \eqref{eq:recursive},    $\Delta(t)=\Delta(t-1)+\underbar{\text{$x$}}_t-c$ for $1\leq t\leq m-1$. Using the initial condition  $\Delta(0)=0$, we get $\Delta(m-1)=\displaystyle\sum_{l=1}^{m-1} \underbar{\text{$x$}}_l-(m-1)c.$
	Using this and \eqref{ineq:fetch_RRE1} we get,
$
	%&\displaystyle\sum_{l=i+1}^{m-1} \underbar{\text{$x$}}_l-(m-i-1)c+\underbar{\text{$x$}}_m-c\geq M,\\ 
	\displaystyle\sum_{l=i+1}^{m} \underbar{\text{$x$}}_l \geq \displaystyle\sum_{l=i+1}^{m} c_l+M.
$
	Thus, RR also fetches at the end of time-slot $m$. Suppose RR fetches the service after the end of time-slot $m'$ for the first time. Therefore by Algorithm \ref{algo:RR},
	$\displaystyle\sum_{l=1}^{m'} \underbar{\text{$x$}}_l \geq \displaystyle\sum_{l=1}^{m'} c_l+M$ and 
	$
	\displaystyle\sum_{l=1}^{t} \underbar{\text{$x$}}_l < \displaystyle\sum_{l=1}^{t} c_l+M.
	$
	for $1\leq t\leq m'-1$.
	Substituting $t=1,2,...m'-1$ successively in the above inequality and using $\Delta(0)=0,$ we get $\Delta(t)<M$ for $1\leq t\leq m'-1$, and
	$
	\Delta(m'-1)+\underbar{\text{$x$}}_m'-c_m'\geq \displaystyle\sum_{l=1}^{m'-1} (\underbar{\text{$x$}}_l-c_l)+\underbar{\text{$x$}}_{m'}-c_{m'}\geq\displaystyle\sum_{l=1}^{m'} (\underbar{\text{$x$}}_{m'}-c_{m'})	\geq M.
$
	Therefore, by \eqref{eq:recursive}, we get $\Delta(m')=M$, which is the  condition for fetching the service under E-RR at the end of time-slot $m'.$
	We thus conclude that the time-slots of first fetch by RR and E-RR are the same.
	
	After the first fetch of service by RR and E-RR at the end of time-slot $m$, let E-RR evict the service at the end of time-slot $n.$
	Therefore by Algorithm \ref{algo:RRE},
	$\Delta(t)\neq 0$ for $m+1\leq t\leq n-1$ and $\Delta(n)=0,$ i.e.,
	\begin{align}\label{ineq:evict_RRE1}
	\Delta(n-1)+\underbar{\text{$x$}}_n-c_n< 0.
	\end{align}
	Since $\Delta(t)\neq 0$ for $m+1\leq t\leq n-1$, from \eqref{eq:recursive},  we have   $\Delta(t)=\min\big\{M,  \Delta(t-1)+\underbar{\text{$x$}}_t-c_t\big\}$ for $m+1\leq t\leq n$.
	Let $j \in [m+1, n-1]$ be a time-slot such that $\Delta(j)=M$ and $\Delta(t)\neq M$ for $j+1 \leq t<n$. Then we get $\Delta(n-1)=\displaystyle\sum_{l=j+1}^{n-1} (\underbar{\text{$x$}}_l-c_l).$
	Using  the condition  $\Delta(m)=M$, we get $\Delta(n-1)= M+\displaystyle\sum_{l=j+1}^{n-1} (\underbar{\text{$x$}}_l-c_l).$
	Using this and \eqref{ineq:evict_RRE1}, we have that,
	$
	%&M+\displaystyle\sum_{l=j+1}^{n-1} \underbar{\text{$x$}}_l-(n-j-1)c+\underbar{\text{$x$}}_n-c<0\\
	%\text{and }&
	\displaystyle\sum_{l=j+1}^{n} \underbar{\text{$x$}}_l +M \leq \displaystyle\sum_{l=j+1}^{n} c_l.
	$
	Thus, RR evicts at the end of time-slot $n.$
	Suppose RR evicts the service after the end of time-slot $n'$ for the first time after $m$. Therefore by Algorithm \ref{algo:RR},
	$\displaystyle\sum_{l=m+1}^{n'} \underbar{\text{$x$}}_l +M \leq \displaystyle\sum_{l=m+1}^{n'} c_l$ and 
	$
	\displaystyle\sum_{l=m+1}^{t} \underbar{\text{$x$}}_l +M > \displaystyle\sum_{l=m+1}^{t} c_l
	$
	for $m+1\leq t\leq n'-1$.
	Substituting $t=m+1,m+2,...n'-1$ successively in the above inequality and using $\Delta(m)=M$, we get $\Delta(t)>0$ for $m+1\leq t\leq n'-1$, i.e., 
	$
	\Delta(n'-1)+\underbar{\text{$x$}}_{n'}-c_{n'}\leq \Delta(m)+ \displaystyle\sum_{l=m+1}^{n'-1} (\underbar{\text{$x$}}_l-c_l)+\underbar{\text{$x$}}_{n'}-c_{n'}
	=M+\displaystyle\sum_{l=m+1}^{n'} (\underbar{\text{$x$}}_{l}-c_l)
	<0.
	$
	Therefore from \eqref{eq:recursive} we get $\Delta(n')=0$, which is the  condition for evicting the service under E-RR at the end of time-slot $n'.$
	Putting together the above results we conclude that the time-slots of first eviction by RR and E-RR are the same. The result then follows by induction.
\end{proof}

\begin{algorithm}
	\caption{Efficient RetroRenting (E-RR)}\label{algo:RRE}
	\SetAlgoLined
	Input: Fetch cost $M$ units, maximum number of our service requests served by edge server($\kappa$),
	renting cost: $c_t$, number of requests: $x_t$, $t > 0$\\
	Output:  Service hosting strategy $r_{t+1}$, $t > 0$\\
	Initialize:  Service hosting variable $r_1 = 0$, $\Delta(0)=0$\\
	\For {\textbf{each} time-slot $t$}{
		$\Delta(t)=\min\Big\{M,\max\big\{0, \Delta(t-1)+\underbar{\text{$x$}}_t-c_t\big\}\Big\}$\\
		\uIf{$\Delta(t)=M$}{
			
			$r_{t+1}=1$\\
		}
		\uElseIf{$\Delta(t)=0$}{ 
			$r_{t+1}=0$\\
		}						
		\Else
		{
			$r_{t+1}=r_t$
		}				
	}
\end{algorithm}
